# Supplementary material for: Multi-level Second-order Few-shot Learning
Source: arXiv:2201.05916 source file (2022-01-15)
Supplement: Supplementary file 1 [file appendix.tex]

\vspace{-0.1cm}
\section{Deriving/Interpreting Pooling via Sigmoid}
\label{sec:pool_der}

Proposition \ref{pr:cooc} and Remark \ref{re:maxexp} state that quantity $1\!-\!(1\!-\!p)^N$ is the probability of at least one co-occurrence being detected in the pool of the $N$ i.i.d. trials performed according to the Bernoulli distribution with the success probability $p$ of event $(\phi_{n}\!\cap\!\phi'_{n}\!=\!1)$ for event vectors in $\vphi,\vphi'\!\!\in\!\{0,1\}^{N}$. Below we extend this theory to negative co-occurrences which we interpret as two anti-correlating visual words.%the case of co-occurrences.
\begin{proposition}
\label{pr:cooc_anti}
Assume an event vector $\vphi^*\!\!\in\!\{0,1,-1\}^{N}$ constructed from event vectors $\vphi,\vphi'\!\!\in\!\{0,1,-1\}^{N}$, which stores the $N$ trials performed according to the Multinomial distribution under i.i.d. assumption, for which the probability $p$ of an event $(\phi^*\!\!=\!\phi_{n}\!\cdot\phi'_{n}\!=\!1)$ denotes a co-occurrence, the probability  $q$ of an event  $(\phi^*\!\!=\phi_{n}\!\cdot\phi'_{n}\!=\!-1)$ denotes a negatively-correlating co-occurrence, and $1\!-\!p\!-\!q$, for $(\phi^*\!\!=\phi_{n}\!\cdot\phi'_{n}\!=0)$ denotes the lack of the first two events, and $p$ is estimated as an expected value $p\!=\!\avg_n\phi^*_n$. Then the probability of at least one co-occurrence event $(\phi^*\!\!=\!1)$ minus the probability of at least one negatively-correlating co-occurrence event $(\phi^*\!\!=\!-1)$ in $N$ trials, encoded in $\phi^*_n$, becomes:
\begin{equation}
\hspace{1cm}
\label{eq:my_maxexp3}
\psi\!=\!(1\!-\!q)^{N}\!-\!(1\!-\!p)^{N}.
\vspace{-0.4cm}
\end{equation}
\end{proposition}
\begin{proof}
One can derive the above difference of probabilities by directly applying the Multinomial calculus as follows:
\vspace{-0.1cm}
\begin{align}
\hspace{0.5cm}
& \!\!\!\!\!\!\!\!\!\!\!\!\!\!\textstyle\sum\limits_{n=1}^{N}\sum\limits_{n'=0}^{N\!-n}\!\!\binom{N}{n,n'\!,N\!-n-n'\!-n''\!}\!\!\left(p^nq^{n'\!}\!-\!p^{n'\!}q^{n}\right)\!(1\!\!-\!\!p\!\!-\!\!q)^{N\!-n-n'}\!.%\nonumber\\[-10pt]
%&
\label{eq:my_maxexppr2}
\end{align}
\vspace{-0.1cm}
One can verify algebraically/numerically that Eq. \eqref{eq:my_maxexppr2} and \eqref{eq:my_maxexp3} are equivalent.% which completes the proof.
\end{proof}

\begin{remark}
%\vspace{-0.3cm}
\label{re:pos_neg_pool}
If we decide from the beginning that the $N$ trials contain only either co-occurrences with the event probability $p\!=\!\rho p'\!$ or negatively-correlating co-occurrences with the event probability $q\!=\!(1\!-\!\rho)q'\!$, we can set $q\!:=\!(1\!-\!\rho)\max(0,-p)$ and $p\!:=\!\rho\max(0,p)$, which leads to:
\vspace{-0.1cm}
\begin{align}
& \psi\!=\!\left(1\!-\!(1\!-\!\rho)\max(0,-p)\right)^N \!\!-\left(1\!-\!\rho\max(0,p)\right)^N\!\!\!,
\label{eq:pos_neg_pool2}
\end{align}
%\vspace{-0.1cm}
%
where $0\!\leq\rho\!\leq\!1$, $-1\!\leq\!p\!\leq\!1$, while $\rho p\!\geq\!0$ and $(1\!-\!\rho) p\!<\!0$ encode the probability of event of co-occurrence and negatively-correlating co-occurrence, respectively.
\end{remark}
\begin{remark}
%\vspace{-0.3cm}
\label{re:pos_neg_pool2r}
%In practice, we trace-normalize $\mM$, $\lambda\!\approx\!1e\!-\!6$, $0\!<\!\eta\!\approx\!N$. Following Remarks \ref{re:pnpn} and \ref{re:maxexp}, $\mPsi\!=\!\mygthree{\,\mM,\eta\,}\!=$
In practice, we trace-normalize $\mM$, use $\lambda\!\approx\!1e\!-\!6$, $0\!<\!\eta\!\approx\!N$, and following Remarks \ref{re:pnpn} and \ref{re:maxexp}, we have:
\begin{align}
\hspace{0.5cm}
& \!\!\!\!\textstyle\mPsi\!=\!\mygthree{\,\mM,\eta\,}\!=
%&\!\!\!\!\!\!\!\!\!\!\!\!\!\!\!\!\!
\!\textstyle\left(1\!-\!(1\!-\!\rho)\max(0,\frac{-\mM}{\trace(\mM)\!+\!\lambda})\right)^\eta \!\!\nonumber\\
&\qquad\qquad\qquad\quad\textstyle
\!\!-\!\!\left(1\!-\!\rho\max(0,\frac{\mM}{\trace(\mM)\!+\!\lambda})\right)^\eta\!\!\!.\!\!
\label{eq:pos_neg_pool3}
\end{align}
\vspace{-0.0cm}
We also apply the soft maximum funct. $\max(\mX,\mY; \alpha)=\frac{1}{\alpha}\log\left(\exp(\alpha \mX)+\exp(\alpha \mY)\right)$ which role is to make derivatives of Eq. \eqref{eq:pos_neg_pool2} and \eqref{eq:pos_neg_pool3} smooth. Lastly, $\alpha$ controls the softness of the max function and $\alpha\!\gg\!\eta$. We call the above operator as MaxExp$\,$({$\pm$}) %$\,$\circled{$\pm$} 
in contrast to MaxExp in Eq. \eqref{eq:my_maxexp3}.
\end{remark}

Figure \ref{fig:power-norms}{\color{red}{a-c}} demonstrates that Eq. \eqref{eq:pos_neg_pool2} and \eqref{eq:pos_neg_pool3} are closely approximated by SigmE from Eq. \eqref{eq:sigmoid} for $\rho\!=\!0.5$. Moreover, derivative of MaxExp$\,$({$\pm$}) with soft maximum is smooth which is essential in back-propagation (non-smooth objectives do not guarantee convergence of the majority of optimization algorithms). As SigmE approximates closely our MaxExp$\,$({$\pm$}), we use SigmE in our experiments. We assert that our relationship descriptors/operators $\vartheta$ benefit from Power Normalization which, according to Prop. \ref{pr:cooc_anti}, can detect co-occurring responses of CNN filters and discards quantities of such responses which correlate with repeatable visual stimuli (\eg~variable areas of textures) which otherwise would introduce nuisance variability into representations. This nuisance variability would be further amplified when learning \eg~pair-wise relations as pairs of images would introduce nuisance quantities $\varepsilon$ and $\varepsilon^*\!$ that would result in a total nuisance variability of $\varepsilon\varepsilon^*\!\!\gg\!\max(\varepsilon,\varepsilon^*\!)$.
